# Supplementary material for: Report on AI-Infused Contouring Workflows for Adaptive Proton Therapy in the Head and Neck
Source: arXiv:2208.04675 source file (2022-09-05)
Supplement: Supplementary file 1 [file appendix-pt-workflow-netherlands.tex]

\chapter{The PT workflow}

Previous work has presented the External Beam Radiotherapy Workflow (EBRT) in detail \cite{TODO}. In this chapter, this work is supplemented with the description of an offline adaptive workflow of a Proton Therapy center in the Netherlands. It results from multiple discussions with participants and careful inspection of internal documents that detail the workflow.

% figure of the complete workflow

\section{Subjects}

Being a complex mesh or processes, there are multiple subjects involved in the PT workflow. Below we list them and their roles in the workflow.
\begin{itemize}
    \item Patient (Pt): individual suffering from a cancer type that might profit from Proton Therapy.
    \item Radiation oncologist (RO): medical doctor specialized in treating cancer with radiation.
    \item Radiotherapy technologist (RTT): highly skilled technician that can perform a diverse set of tasks in the RT pipeline. They can have multiple roles depending on their skill set (earned through in-site training).
    \begin{itemize}
        \item Dose planning: trained in operating the software that is used to create treatment plans as well as in the methods for assessing them such as reading dose volume histograms and setting structure specific constraints. 
        \item Gantry: trained in operating the gantry's hardware and software which depends on the manufacturer of the treatment machine. Gantry RTTs should also know how to operate portal imaging to perform IGRT.
        \item Imaging: trained in operating image acquisition hardware such as CT, PET/CT and MR scanners. 
    \end{itemize}
    \item Medical physicist (MP): in charge of making sure that all the pipeline works appropriately and consistently. 
    \item Care coach: in charge of walking the patient through the treatment dealing with administrative issues such as registration and data management.
    \item Capacity planner: assesses whether there is capacity in the Proton Therapy center for the incoming patient. 
\end{itemize}

\section{Diagnosis and referral}

The first step of the patient's journey is the diagnosis, which includes determining the type of tumor and whether it is suitable for EBRT. Given the limited capacity of PT centers, an external RO is in charge of performing the initial assessment and diagnosis. If they consider that the patient's tumor can be treated with EBRT and that they might benefit from PT, then several things happen. 

First, a regular photon-based treatment plan 

they can refer them to a PT center. Before accepting the patient, the capacity planner of the PT center makes sure that there are enough resources to treat 

Given that PT is a recent treatment modality, there is still a limited capacity. Therefore, patients first go to an external 

Given the limited number of PT centers, in the Netherlands  there is a 

In the Netherlands, the patient's process starts 

\section{}

\section{Treatment creation}

\section{Treatment delivery}

\section{Follow-up}
